# Supplementary material for: Graph Neural Networks as a Substitute for Transformers in Single-Cell Transcriptomics
Source: arXiv:2507.04125 source file (2025-07-05)
Supplement: Supplementary file 1 [file 7.appendix.tex]

This supplementary material provides additional details for the main paper, including \textit{A. More Method Details}, where we provide further deductions for Eq.(14) in the main paper to illustrate the essential difference between Transformers and GNNs, \textit{B. Dataset and Implementation Details}, where we provide further introductions for the transcriptomic datasets and our experimental implementations, \textit{C. More Experiments and Discussions}, where we provide more details for Table~1 and Figure~4 in the main paper and further discussions, such as the reason for the mixed usage of the concepts `positions' and `relative positions'.

% \section*{Appendix}
\section*{A. More Method Details}
% \medskip

\noindent\textbf{Preliminaries.} 

% \smallskip
For the dataset, \eg, trancriptomics, $\mathcal{D}\!=\!\{(\bm{x}_i, \bm{v}_i)\}_{i=1}^N$, where $(\bm{x}_i, \bm{v}_i) = (x_{i,1}, x_{i,2}, \ldots, x_{i,l}; v_{i,1}, v_{i,2}, \ldots, v_{i,l})$. The  masked value input is $(\bm{x}_i, \tilde{\bm{v}}_i) = (x_{i,1}, x_{i,2}, \ldots, x_{i,l}$; $v_{i,1}, [mask], \ldots, v_{i,l})$.
We first re-write the masked value prediction loss, \ie, Eq.~(5) in the main paper, here:
\begin{gather}
\label{supp:base_objective}
\mathcal{L}_{\text{\textit{MVP}}}(\mathcal{D}, \theta) = \frac{1}{N} \sum_{i=1}^N \sum_{k} \left\|v_{i,k} - f((\bm{x}_i, \tilde{\bm{v}}_i), \theta)_k\right\|^2, \tag{a}
\end{gather}
%---------------------------------
where $v_{i,k}$ is the $k$-th masked value in $\tilde{\bm{v}}_i$ and $f((\bm{x}_i, \tilde{\bm{v}}_i), \theta)_k$ represents the corresponding predicted value.

We assume that position \textbf{exists} in this dataset (not the real case in transcriptomics). For the calculation of $f((\bm{x}_i, \tilde{\bm{v}}_i), \theta)_k$, the whole process can be written as:
\begin{gather}
\label{supp:embed_process}
\bm{e} = \mathbf{E_\theta}(\bm{x}_i) + \mathbf{L_{1,\theta}}(\tilde{\bm{v}}_i) + \bm{p}, \tag{b} \\
\label{supp:feature_extraction}
\bm{e}' = (e'_1, e'_2, \ldots, e'_l) = \mathbf{M_\theta}(\bm{e}), \tag{c}\\
\label{supp:value_prediction}
f((\bm{x}_i, \tilde{\bm{v}}_i), \theta)_k = \mathbf{L_{2,\theta}}(e'_k), \tag{d}
\end{gather}
where $\bm{p}=(p_1,p_2,\ldots,p_l)$ is the (absolute) positional embedding and $l$ is the sequence length, other symbols serve as the same roles described in Eq.~(6) to Eq.~(8) in the main paper.

For convenience, we assume there is only one layer of Transformer and GNN, and the feature extraction process for the two models could be re-written as:
\begin{gather}
\bm{e}'_{tf} = \text{\text{Softmax}}\left((\bm{e}\mathbf{w}_Q )(\bm{e}\mathbf{w}_K )^T\right) (\bm{e}\mathbf{w}_V ), \tag{e}\\
\bm{e}'_{gnn} = \text{Softmax}(\mathbf{A}) \bm{e}, \tag{f}
\end{gather}
where the symbols serve the same roles described in Eq.~(9) and Eq.~(11) in the main paper.

\medskip
\noindent\textbf{Comparisons of Empirical Risks.} 
\smallskip

We still apply the assumption in the main paper, that value is defined as the summation of the influence of token, other values, and other values considering relative positions:
\begin{align}
\label{value_gen_func_app}
 v_k = h_1(x_k) + {\textstyle\sum_j} h_2(v_j) + {\textstyle\sum_j} h_3(p_{kj}v_j), \tag{g}
\end{align}
where $h_1$, $h_2$ and $h_3$ are inherent functions for value generation, $j$ indexes all tokens except $k$ in the sample, $p_{kj}$ is the relative positions between $k$ and $j$. Considering the difference between $h_2$ and $h_3$, where the first function aggregates the influence from other values without considering their relative positions. Therefore, when $p_{kj} = 0$ or the influence from associated values $v_j$ to $v_k$ remains constant, $h_3$ effectively performs the same function as $h_2$, \ie, these two functions can be merged. This rationale supports our claim that under certain conditions, function $h_3$ will degenerate to $h_2$ in the main paper.

Assuming that Transformers and GNNs have a similar ability to learn $h_1$ and $h_2$, the difference generated from the training empirical risk (not the generalization risk), Eq.~(14) in the main paper:
\begin{align}
 \mathcal{R}_{h_3} &= {\textstyle\sum_{\mathcal{D}}\sum_j} \|h_3(p_{kj}v_j) - f(p_{kj},v_j)\|^2. \tag{h}
\end{align}

For any two specific tokens $x_k$ and $x_j$, the influence from $x_j$ to $x_k$ varies in response to $p_{kj} \in \mathcal{P}$, encoded by $h_3$, where $\mathcal{P}$ represents the set for all possible values of relative positions. Without loss of generality, by only considering two tokens (the values of $k$ and $j$ could change but tokens $x_k$ and $x_j$ are unchanged) and the effect from $x_j$ to $x_k$ across all samples, $h_3$ as a static coefficient and $g_\theta$ is the optimization target, the risk could be further written as:
\begin{align}
 \mathcal{R}_{h_3,x_j\rightarrow x_k} &= {\textstyle\sum_{\mathcal{D}}} \|h_3p_{kj}v_j - g_\theta v_j\|^2, \tag{i}\\
 &= {\textstyle\sum_{\mathcal{D}}} \|h_3p_{kj} - g_\theta\|^2  \|v_j\|^2. \tag{j}
\end{align}
where $g_\theta$ is the function of $s_{kj}$, where $s_{kj} = (e_k\mathbf{w_Q} ) (e_j\mathbf{w_K} )^T$ for Transformer. Since $e_k$ and $e_j$ encode position $p_k$ and $p_j$ as described in Eq.~\eqref{supp:embed_process}, the optimum for Transformer is $g_\theta^*=h_3(p_k-p_j)=h_3p_{kj}$ and the optimal risk is 0. On the other hand, for GNNs, as its $g_\theta$ does not accept $p_k$ and $p_j$ as input, it can only learn a constant for various $p_{kj}$ from the optimization, and its optimum should be $g_\theta^*=h_3\mathbb{E}\left[p_{kj}\right]$. Given the above discussion, the training risk difference between optimal Transformer and GNN could be written as:
\begin{align}
 \mathcal{R}_{h_3,\Delta} &= {\textstyle\sum_{\mathcal{D}}\sum_j} \|p_{kj} - \mathbb{E}\left[p_{kj}\right]\|^2  \|h_3 v_j\|^2, \tag{k}
\end{align}
where the optimal loss of Transformers is 0 and Eq.~(k) is also the optimal loss for GNN, $\Delta$ denotes the difference between the two models.

Based on the discussions above, we find that if $p_{kj}$ is a constant, (\ie, $p_{kj} = \mathbb{E}\left[p_{kj}\right] = c$, where $c$ is a constant) or even $p_{kj}=0$, the risk difference $\mathcal{R}_{h_3,\Delta}$ is equal to 0, which confirms our hypothesis that Transformers and GNNs are equivalent. To further verify the inherent discrepancy between GNNs and Transformers lies in their ability to handle relative positions, we conducted synthetic experiments and large-scale experiments in the main paper.

\section*{B. Dataset and Implementation Details}

% \medskip
\noindent\textbf{More Dataset Details.}

% \smallskip

Single-cell transcriptomics, abbreviated as transcriptomics in the main paper, leverages high-throughput technologies to sequence and analyze RNA from individual cells \cite{kolodziejczyk2015technology}. This method facilitates essential biological tasks such as cell annotation and perturbation prediction. Transcriptomic data typically comprise a sequence-like dataset without positions (\ie, no relative orders between genes), represented as a set of genes and their associated expression values: $(\text{gene}_1, \text{gene}_2, \ldots, \text{gene}_n)$,$ (\text{expr}_1, \text{expr}_2, \ldots, \text{expr}_n)$, where $\text{expr}$ denotes the associated expression values. In transcriptomics, each gene appears only once, and there are no relative orders between genes, \textit{i.e.}, no positions nor relative positions. Due to its sequence-like data structure, many researchers have conducted extensive Transformer-based pretraining on large-scale transcriptomic datasets, consuming significant resources, especially when gene length is extremely large. Therefore, exploring the potential of Graph Neural Networks as an alternative for Transformers in this field, \ie, where the dataset lacks positions, is of significant interest.

We follow the dataset settings and pre-training downstream verification procedure applied in scGPT~\cite{scGPT} to assemble a large-scale transcriptomic dataset for the self-supervised pre-training of our benchmark and five downstream transcriptomic classification datasets. The pre-training dataset comprises single-cell RNA transcriptomics from 54.6 million human cells, which is sourced from the CELLxGENE~\cite{czi2023cz} collection. It includes samples from about 51 organs and tissues (e.g., heart, blood, and brain) derived from more than 441 studies, offering extensive coverage of cellular heterogeneity throughout the human body. The five downstream datasets feature fewer transcriptomic samples but include class labels, such as cell type and disease type, making them suitable for validating the effectiveness of the pre-trained models. Here, we introduce the five transcriptomic datasets in detail:

Leptomeningeal (Lept)~\cite{remsik2023leptomeningeal}, which identifies that leptomeningeal-specific IFN-$\gamma$ signaling plays a pivotal role in cancer cell growth independently of adaptive immunity and suggests a novel immunotherapeutic strategy targeting tumors. This dataset consists of 20,676 cells and includes 10 classes, such as CD4 T cell, CD8 T cell, etc.

Sclerosis~\cite{schirmer2019neuronalMS}, which reveals specific cellular changes in multiple sclerosis lesions, highlighting the roles of neuron damage and glial activation in driving disease progression, which consists of 21,312 cells and 18 classes, such as pyramidal neurons, phagocytes, etc.

Pancreas~\cite{chen2023transformerPanc}, which aggregates data from five human pancreas studies for cell type annotation tasks. This dataset consists of 14,818 cells and includes 14 classes, such as T-cell, ductal, etc.

Lupus~\cite{perez2022single}, which identifies increased type 1 interferon-stimulated genes in monocytes, accompanied by a reduction in naive CD4 T cells and an expansion of cytotoxic GZMH CD8 T cells. This dataset consists of 79,322 cells (we randomly select 50,000 samples among those) and includes 14 classes, such as T4-reg, NK-dim, etc.

Dengue~\cite{ghita2023global}, which identifies the target cells of the dengue virus, including myeloid cells and B cells, and outlines the immunological characteristics of severe dengue progression in children's blood. This dataset consists of 193,727 cells (we randomly select 50,000 samples among those) and includes 23 classes, such as CD8+ naive T cells, CD4+ naive T cells, etc.

\noindent\textbf{More Implementation Details.} 
\noindent\textbf{Further Discussions.}
\begin{figure*}[t!]
\centering\includegraphics[width=\linewidth]{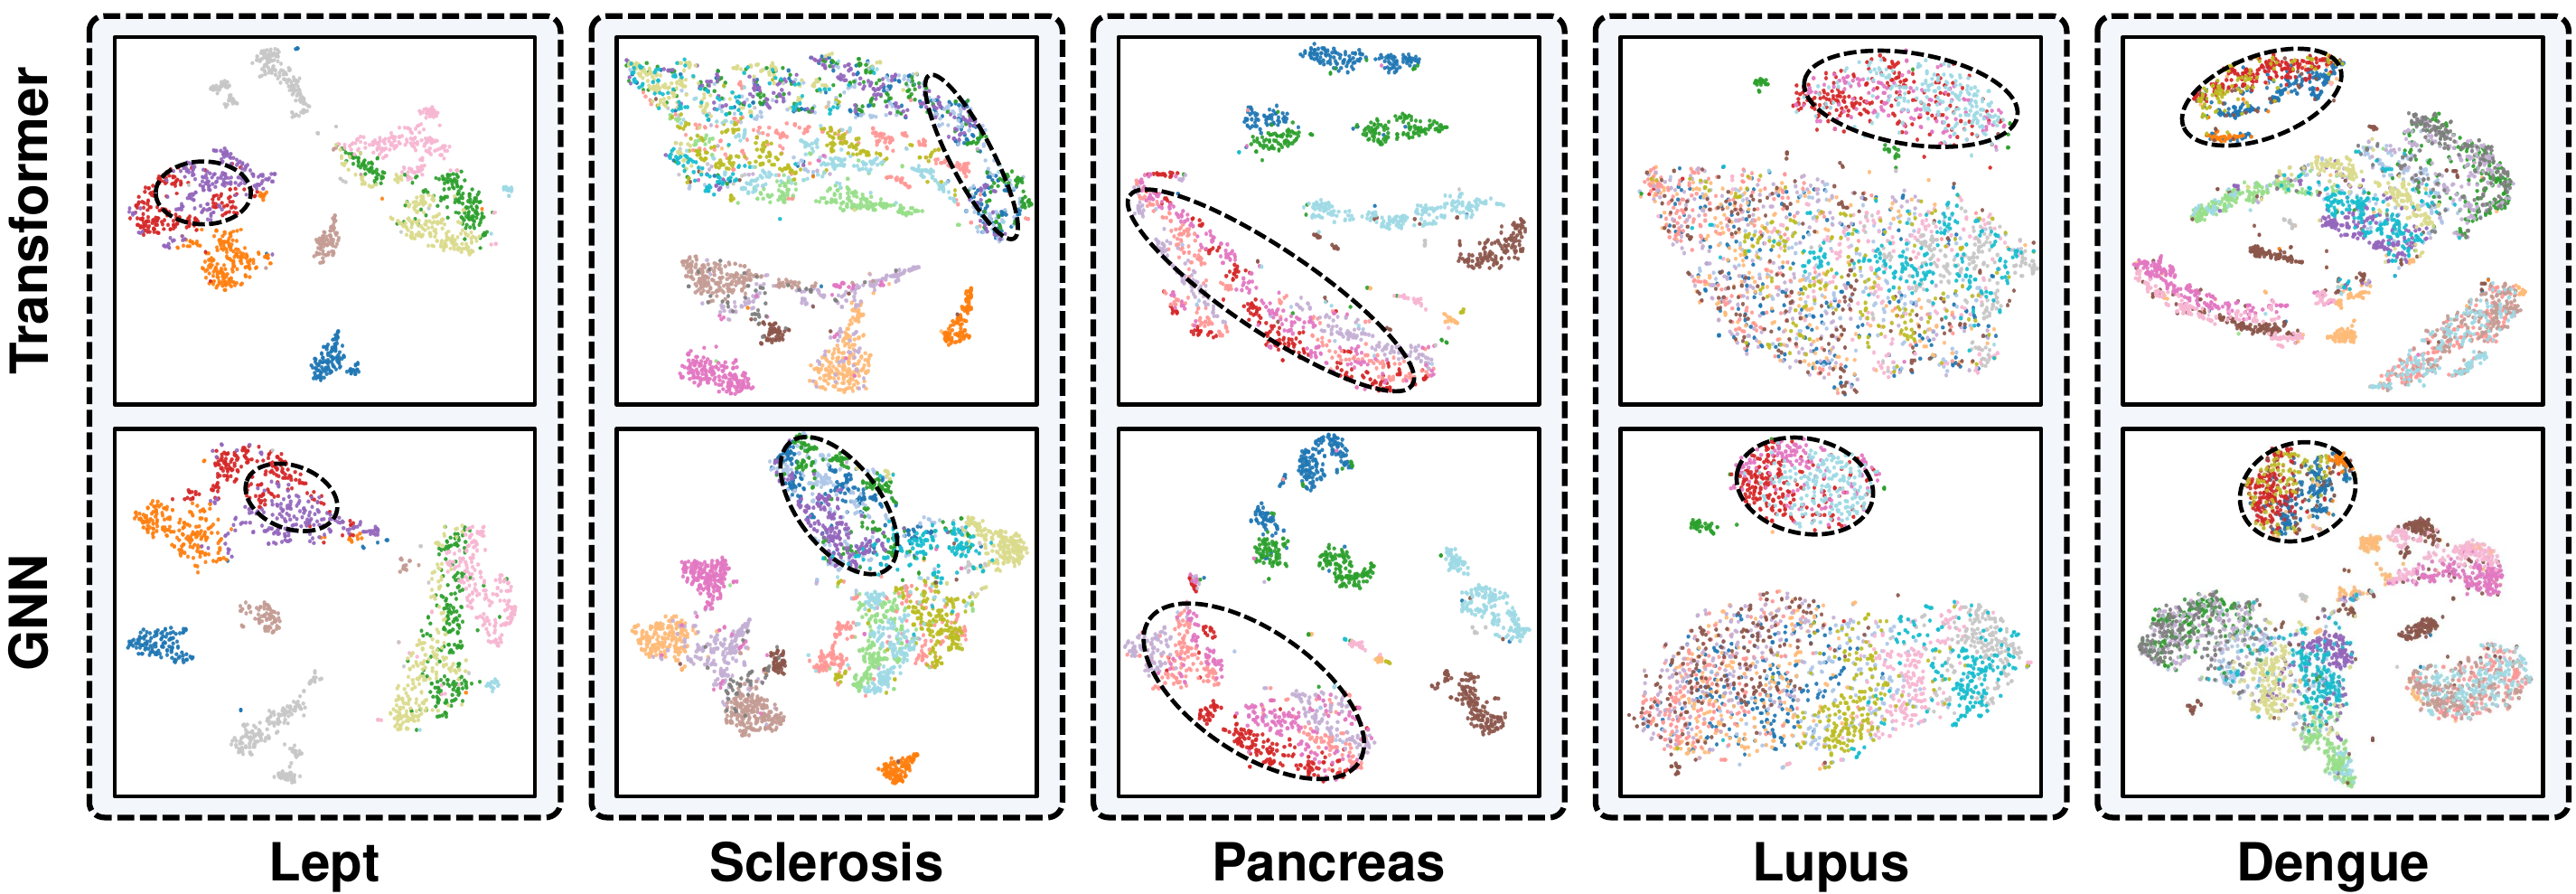}
    % \vspace{-4pt}
    \caption{Supplementary for Figure~4 in the main paper. t-SNE~\cite{van2008visualizing} visualization of features extracted by Transformers (Top) and GNNs (Bottom) across five transcriptomic datasets. For each dataset, all classes are displayed, and black dashed circles highlight areas where both models exhibit similar confusion.}
    % \vspace{-8pt}
    \label{supp:tsne}
\end{figure*}
% \smallskip
To ensure fair comparisons, both GNNs and Transformers were configured under uniformly applied experimental settings, including a 6-layer model structure,  a hidden dimension size of 256, a batch size of 256, an input gene length set as 512, and 10 training epochs. An Adam optimizer with a learning rate of 0.0002 was employed during pre-training. For GNNs, due to the lack of a pre-defined graph, the adjacency matrix $\mathbf{A}$ was modeled as a trainable matrix. Note that since the gene dictionary is extremely large, reaching up to $60,000$, optimizing such an adjacency matrix is clearly impractical. Therefore, we employed a commonly used matrix factorization method, optimizing two matrices of size $d \times s$, where $s$ represents the size of the gene dictionary and $d=48$ is the dimension for the reduced feature space, significantly reducing the number of parameters. The feature extractor was frozen for downstream classification tasks, and a single linear layer was trained as the classifier to fully evaluate pre-training performance. The downstream datasets were split into 70\% as the training set and 30\% as the testing set. We applied the settings, including 50 training epochs, and a batch size of 64, using the Adam optimizer with a learning rate of 0.005 for evaluating both of the two models. Each experiment was independently replicated five times using the same hardware, with the averaged results subsequently reported.

\section*{C. More Experiments and Discussions}

% \medskip
\noindent\textbf{More Experimental Results.}
\begin{table}[t]
\centering
\caption{Supplementary for Table~1 in the main paper with \textbf{no positional encoding} settings, \ie, $\alpha=0$ in Eq.~(15) in the main paper, note that such setting is only a synthetic setting and unlikely to occur in real data. Comparisons of test losses in synthetic example between Transformers and GNNs with varying $e_p$ and $\sigma$. $r_\Delta\!=\! \mathcal{L}_{GNN}/\mathcal{L}_{TF}$ indicates the relative loss differences between them. Avg denotes the averaged result across $\sigma$. For $r_\Delta$, a larger number denotes Transformer is better, and for others, a smaller number is better.}
    
     \scalebox{1.0}{
\begin{tabular}{c|c|ccccc|c}

\toprule
\(e_p \backslash \sigma\)  &  & 0.1 & 0.2 & 0.3 & 0.4 & 0.5 & Avg \\ 
 \hline
\multirow{3}{*}{0} & TF & 0.009 & 0.034 & 0.075 & 0.136 & 0.208 & -   \\
&GNN         &  0.013 & 0.039 & 0.083 & 0.145 & 0.224 & -\\
& $r_\Delta$  & 1.444 & 1.147 & 1.107 & 1.066 & 1.077 & 1.168 \\
\hline
\multirow{3}{*}{0.1} & TF & 0.008 & 0.033 & 0.068 & 0.119 & 0.186 & -\\
&GNN         & 0.024 & 0.054 & 0.097 & 0.162 & 0.248 & -\\
& $r_\Delta$  & 3.000 & 1.636 & 1.426 & 1.361 & 1.333 & 1.752 \\
\hline
\multirow{3}{*}{0.2} & TF & 0.009 & 0.027 & 0.063 & 0.134 & 0.205 & - \\
&GNN         &0.037 & 0.071 & 0.128 & 0.205 & 0.298 & - \\
& $r_\Delta$  &4.111 & 2.630 & 2.032 & 1.530 & 1.454 & 2.351 \\
\hline
\multirow{3}{*}{0.3} & TF &  0.015 & 0.030 & 0.064 & 0.139 & 0.199 & - \\
&GNN         & 0.073 & 0.112 & 0.185 & 0.280 & 0.407 & -\\
& $r_\Delta$  & 4.867 & 3.733 & 2.891 & 2.014 & 2.045 & 3.110 \\
\hline
\multirow{3}{*}{0.4} & TF& 0.016 & 0.031 & 0.057 & 0.136 & 0.194 & - \\
&GNN         & 0.124 & 0.180 & 0.282 & 0.420 & 0.589 & -\\
& $r_\Delta$  & 7.750 & 5.806 & 4.947 & 3.088 & 3.036 & 4.926 \\
\hline
\multirow{3}{*}{0.5} & TF& 0.012 & 0.050 & 0.089 & 0.133 & 0.191 & -\\
&GNN         &0.206 & 0.297 & 0.439 & 0.621 & 0.882 & - \\
& $r_\Delta$  &17.167 & 5.940 & 4.933 & 4.669 & 4.618 & 7.465 \\
% \hline

\bottomrule
\end{tabular}
}

\label{supp:toy_table_no_pos}
% \vspace{-8pt}
\end{table}

% \smallskip
We provide more details in Table~\ref{supp:toy_table_no_pos} and Figure~\ref{supp:tsne} as supplements to Table~1 and Figure~4, respectively, which further demonstrate our conclusions in the main paper.

In Table~\ref{supp:toy_table_no_pos} we show the results where there are no (absolute) positional encoding, and we find there is no change in the results and our conclusions, which means such positional encoding does not influence the optimization of two models. Note that we set the position coefficient $\alpha$ not equal to 0 in the main paper because we would like to show the difference between GNNs and Transformers is purely caused by the relative positions, and we do not want to mix its effect into the whole position effect. The configurations in the main paper are better suited to support our conclusions than the experimental settings described in Table~\ref{supp:toy_table_no_pos}.

% \medskip

% \smallskip
\noindent\textit{Q1.} \textit{Why do we sometimes use the term `positions' and sometimes use the term `relative positions'?}

First, the concept of `positions' is not synonymous with `relative positions', although they are closely related. Specifically, `relative positions' is implied within `positions'; that is, without order defined by `positions', there is no basis for `relative positions'. On the other hand, `positions' without `relative positions' lack practical examples currently and exist only as theoretical constructs, such as our designed synthetic example when \(e_p = 0\). As mentioned in the title, our investigation focuses on the equivalence of GNNs and Transformers when `positions' are absent. However, we found that the key differences and equivalences are determined by the presence or absence of `relative positions'. Thus, our title could be revised to `Graph Neural Networks are Equivalent to Transformers without Relative Positions'. Yet, considering that the only method to remove `Relative Positions' in real datasets involves discarding `positions` entirely, \eg, in transcriptomics, extending the equivalence to also encompass `positions' is valid.

% \smallskip
\noindent\textit{Q2.} \textit{What is the difference between our proposed GNN implementation and a Transformer equipped with global attention?}

As written in our implementation details for GNNs, we utilized an optimizable adjacency matrix to implement the attention mechanism for feature interaction in GNNs, rather than relying on the pre-defined graph structure, as there is no inherent graph among genes. Therefore, if the QKV attention of Transformers is replaced with trainable global attention weights among nodes, these two models' implementations become entirely the same.
However, it is critical to note that the superiority of the Transformers comes from the dynamic QKV attention and such replacement will raise the question of whether it can still be called Transformers. 
Furthermore, such similarity between the implementations of GNNs and Transformers further proves the fundamental resemblance between the two models and forms the basis of their equivalence under specific settings, \ie, no positions.
As for the validity of the trainable graph implementation in GNNs, if a set of nodes indeed has a graph structure, then using optimizable parameters as the edges for learning can achieve the optimal configuration of that graph. Consequently, the optimizable graph structure effectively becomes equivalent to the inherent graph structure. This suggests that our implementation is valid when the graph is unknown unless biases in the training data influence the optimization of the trainable graph, which lies outside the scope of our discussions.

% \smallskip
\noindent\textit{Q3.} \textit{Why was transcriptomics selected for our large-scale experimental verification?}

First, because it typically represents sequence-like data without positions and is of a large scale, such magnitudes and suitability are not yet observed in other fields. 
Second, the extensive applications of large-scale Transformer pre-training in this field have consumed a significant amount of computational resources, despite some attempts to conserve resources through more efficient Transformer modifications~\cite{scFoundation}, which have achieved only minimal success.
The equivalence between GNNs and Transformers under the settings we proposed addresses this pressing problem, providing crucial advancements in the field. Finally, transcriptomics is a suitable example we have identified, and our conclusions are substantiated by synthetic experiments, ensuring that they can be generalized to any dataset without positions.
