# Supplementary material for: Graph Neural Networks as a Substitute for Transformers in Single-Cell Transcriptomics
Source: arXiv:2507.04125 source file (2025-07-05)
Supplement: Supplementary file 2 [file supp_dataset.tex]

Single-cell transcriptomics, abbreviated as transcriptomics in the main paper, leverages high-throughput technologies to sequence and analyze RNA from individual cells \cite{kolodziejczyk2015technology}. This method facilitates essential biological tasks such as cell annotation and perturbation prediction. Transcriptomic data typically comprise a sequence-like dataset without positions (\ie, no relative orders between genes), represented as a set of genes and their associated expression values: $(\text{gene}_1, \text{gene}_2, \ldots, \text{gene}_n)$,$ (\text{expr}_1, \text{expr}_2, \ldots, \text{expr}_n)$, where $\text{expr}$ denotes the associated expression values. In transcriptomics, each gene appears only once, and there are no relative orders between genes, \textit{i.e.}, no positions nor relative positions. Due to its sequence-like data structure, many researchers have conducted extensive Transformer-based pretraining on large-scale transcriptomic datasets, consuming significant resources, especially when gene length is extremely large. Therefore, exploring the potential of Graph Neural Networks as an alternative for Transformers in this field, \ie, where the dataset lacks positions, is of significant interest.

We follow the dataset settings and pre-training downstream verification procedure applied in scGPT~\cite{scGPT} to assemble a large-scale transcriptomic dataset for the self-supervised pre-training of our benchmark and five downstream transcriptomic classification datasets. The pre-training dataset comprises single-cell RNA transcriptomics from 54.6 million human cells, which is sourced from the CELLxGENE~\cite{czi2023cz} collection. It includes samples from about 51 organs and tissues (e.g., heart, blood, and brain) derived from more than 441 studies, offering extensive coverage of cellular heterogeneity throughout the human body. The five downstream datasets feature fewer transcriptomic samples but include class labels, such as cell type and disease type, making them suitable for validating the effectiveness of the pre-trained models. Here, we introduce the five transcriptomic datasets in detail:

Leptomeningeal (Lept)~\cite{remsik2023leptomeningeal}, which identifies that leptomeningeal-specific IFN-$\gamma$ signaling plays a pivotal role in cancer cell growth independently of adaptive immunity and suggests a novel immunotherapeutic strategy targeting tumors. This dataset consists of 20,676 cells and includes 10 classes, such as CD4 T cell, CD8 T cell, etc.

Sclerosis~\cite{schirmer2019neuronalMS}, which reveals specific cellular changes in multiple sclerosis lesions, highlighting the roles of neuron damage and glial activation in driving disease progression, which consists of 21,312 cells and 18 classes, such as pyramidal neurons, phagocytes, etc.

Pancreas~\cite{chen2023transformerPanc}, which aggregates data from five human pancreas studies for cell type annotation tasks. This dataset consists of 14,818 cells and includes 14 classes, such as T-cell, ductal, etc.

Lupus~\cite{perez2022single}, which identifies increased type 1 interferon-stimulated genes in monocytes, accompanied by a reduction in naive CD4 T cells and an expansion of cytotoxic GZMH CD8 T cells. This dataset consists of 79,322 cells (we randomly select 50,000 samples among those) and includes 14 classes, such as T4-reg, NK-dim, etc.

Dengue~\cite{ghita2023global}, which identifies the target cells of the dengue virus, including myeloid cells and B cells, and outlines the immunological characteristics of severe dengue progression in children's blood. This dataset consists of 193,727 cells (we randomly select 50,000 samples among those) and includes 23 classes, such as CD8+ naive T cells, CD4+ naive T cells, etc.
