# Supplementary material for: Graph Neural Networks as a Substitute for Transformers in Single-Cell Transcriptomics
Source: arXiv:2507.04125 source file (2025-07-05)
Supplement: Supplementary file 3 [file supp_method.tex]

\noindent\textbf{Preliminaries.} 

% \smallskip
For the dataset, \eg, trancriptomics, $\mathcal{D}\!=\!\{(\bm{x}_i, \bm{v}_i)\}_{i=1}^N$, where $(\bm{x}_i, \bm{v}_i) = (x_{i,1}, x_{i,2}, \ldots, x_{i,l}; v_{i,1}, v_{i,2}, \ldots, v_{i,l})$. The  masked value input is $(\bm{x}_i, \tilde{\bm{v}}_i) = (x_{i,1}, x_{i,2}, \ldots, x_{i,l}$; $v_{i,1}, [mask], \ldots, v_{i,l})$.
We first re-write the masked value prediction loss, \ie, Eq.~(5) in the main paper, here:
\begin{gather}
\label{supp:base_objective}
\mathcal{L}_{\text{\textit{MVP}}}(\mathcal{D}, \theta) = \frac{1}{N} \sum_{i=1}^N \sum_{k} \left\|v_{i,k} - f((\bm{x}_i, \tilde{\bm{v}}_i), \theta)_k\right\|^2, \tag{a}
\end{gather}
%---------------------------------
where $v_{i,k}$ is the $k$-th masked value in $\tilde{\bm{v}}_i$ and $f((\bm{x}_i, \tilde{\bm{v}}_i), \theta)_k$ represents the corresponding predicted value.

We assume that position \textbf{exists} in this dataset (not the real case in transcriptomics). For the calculation of $f((\bm{x}_i, \tilde{\bm{v}}_i), \theta)_k$, the whole process can be written as:
\begin{gather}
\label{supp:embed_process}
\bm{e} = \mathbf{E_\theta}(\bm{x}_i) + \mathbf{L_{1,\theta}}(\tilde{\bm{v}}_i) + \bm{p}, \tag{b} \\
\label{supp:feature_extraction}
\bm{e}' = (e'_1, e'_2, \ldots, e'_l) = \mathbf{M_\theta}(\bm{e}), \tag{c}\\
\label{supp:value_prediction}
f((\bm{x}_i, \tilde{\bm{v}}_i), \theta)_k = \mathbf{L_{2,\theta}}(e'_k), \tag{d}
\end{gather}
where $\bm{p}=(p_1,p_2,\ldots,p_l)$ is the (absolute) positional embedding and $l$ is the sequence length, other symbols serve as the same roles described in Eq.~(6) to Eq.~(8) in the main paper.

For convenience, we assume there is only one layer of Transformer and GNN, and the feature extraction process for the two models could be re-written as:
\begin{gather}
\bm{e}'_{tf} = \text{\text{Softmax}}\left((\bm{e}\mathbf{w}_Q )(\bm{e}\mathbf{w}_K )^T\right) (\bm{e}\mathbf{w}_V ), \tag{e}\\
\bm{e}'_{gnn} = \text{Softmax}(\mathbf{A}) \bm{e}, \tag{f}
\end{gather}
where the symbols serve the same roles described in Eq.~(9) and Eq.~(11) in the main paper.

\medskip
\noindent\textbf{Comparisons of Empirical Risks.} 
\smallskip

We still apply the assumption in the main paper, that value is defined as the summation of the influence of token, other values, and other values considering relative positions:
\begin{align}
\label{value_gen_func_app}
 v_k = h_1(x_k) + {\textstyle\sum_j} h_2(v_j) + {\textstyle\sum_j} h_3(p_{kj}v_j), \tag{g}
\end{align}
where $h_1$, $h_2$ and $h_3$ are inherent functions for value generation, $j$ indexes all tokens except $k$ in the sample, $p_{kj}$ is the relative positions between $k$ and $j$. Considering the difference between $h_2$ and $h_3$, where the first function aggregates the influence from other values without considering their relative positions. Therefore, when $p_{kj} = 0$ or the influence from associated values $v_j$ to $v_k$ remains constant, $h_3$ effectively performs the same function as $h_2$, \ie, these two functions can be merged. This rationale supports our claim that under certain conditions, function $h_3$ will degenerate to $h_2$ in the main paper.

Assuming that Transformers and GNNs have a similar ability to learn $h_1$ and $h_2$, the difference generated from the training empirical risk (not the generalization risk), Eq.~(14) in the main paper:
\begin{align}
 \mathcal{R}_{h_3} &= {\textstyle\sum_{\mathcal{D}}\sum_j} \|h_3(p_{kj}v_j) - f(p_{kj},v_j)\|^2. \tag{h}
\end{align}

For any two specific tokens $x_k$ and $x_j$, the influence from $x_j$ to $x_k$ varies in response to $p_{kj} \in \mathcal{P}$, encoded by $h_3$, where $\mathcal{P}$ represents the set for all possible values of relative positions. Without loss of generality, by only considering two tokens (the values of $k$ and $j$ could change but tokens $x_k$ and $x_j$ are unchanged) and the effect from $x_j$ to $x_k$ across all samples, $h_3$ as a static coefficient and $g_\theta$ is the optimization target, the risk could be further written as:
\begin{align}
 \mathcal{R}_{h_3,x_j\rightarrow x_k} &= {\textstyle\sum_{\mathcal{D}}} \|h_3p_{kj}v_j - g_\theta v_j\|^2, \tag{i}\\
 &= {\textstyle\sum_{\mathcal{D}}} \|h_3p_{kj} - g_\theta\|^2  \|v_j\|^2. \tag{j}
\end{align}
where $g_\theta$ is the function of $s_{kj}$, where $s_{kj} = (e_k\mathbf{w_Q} ) (e_j\mathbf{w_K} )^T$ for Transformer. Since $e_k$ and $e_j$ encode position $p_k$ and $p_j$ as described in Eq.~\eqref{supp:embed_process}, the optimum for Transformer is $g_\theta^*=h_3(p_k-p_j)=h_3p_{kj}$ and the optimal risk is 0. On the other hand, for GNNs, as its $g_\theta$ does not accept $p_k$ and $p_j$ as input, it can only learn a constant for various $p_{kj}$ from the optimization, and its optimum should be $g_\theta^*=h_3\mathbb{E}\left[p_{kj}\right]$. Given the above discussion, the training risk difference between optimal Transformer and GNN could be written as:
\begin{align}
 \mathcal{R}_{h_3,\Delta} &= {\textstyle\sum_{\mathcal{D}}\sum_j} \|p_{kj} - \mathbb{E}\left[p_{kj}\right]\|^2  \|h_3 v_j\|^2, \tag{k}
\end{align}
where the optimal loss of Transformers is 0 and Eq.~(k) is also the optimal loss for GNN, $\Delta$ denotes the difference between the two models.

Based on the discussions above, we find that if $p_{kj}$ is a constant, (\ie, $p_{kj} = \mathbb{E}\left[p_{kj}\right] = c$, where $c$ is a constant) or even $p_{kj}=0$, the risk difference $\mathcal{R}_{h_3,\Delta}$ is equal to 0, which confirms our hypothesis that Transformers and GNNs are equivalent. To further verify the inherent discrepancy between GNNs and Transformers lies in their ability to handle relative positions, we conducted synthetic experiments and large-scale experiments in the main paper.
